# Supplementary material for: What Makes Multimodal In-Context Learning Work?
Source: arXiv:2404.15736 source file (2024-04-25)
Supplement: Supplementary file 1 [file X_suppl.tex]

\clearpage
\setcounter{page}{1}
\maketitlesupplementary
\include{sec/7_annex}
